# Supplementary material for: NanoGS: Training-Free Gaussian Splat Simplification
Source: arXiv:2603.16103 source file (2026-09-01)
Supplement: Supplementary file 2 [file supplementary.tex]

% Requires: \usepackage{booktabs,multirow}
\begin{table*}[t]
\centering
\setlength{\tabcolsep}{6pt}

\small
\begin{tabular}{llcccccc}
\toprule
PSNR/Num($k$)/Mem(MB) & $p$  & 0.8 & 0.6 & 0.4 & 0.3 & 0.2 & 0.1 \\
\midrule
\multirow{3}{*}{NeRF} 
& Scene1 & xx.xx & xx.xx & xx.xx & xx.xx & xx.xx & xx.xx \\
& Scene1 & xx.xx & xx.xx & xx.xx & xx.xx & xx.xx & xx.xx \\
& Scene1 & xx.xx & xx.xx & xx.xx & xx.xx & xx.xx & xx.xx \\
& Scene1    & xx.xx & xx.xx & xx.xx & xx.xx & xx.xx & xx.xx \\
\midrule
\multirow{3}{*}{M360}
& Scene1 & xx.xx & xx.xx & xx.xx & xx.xx & xx.xx & xx.xx \\
& Scene1 & xx.xx & xx.xx & xx.xx & xx.xx & xx.xx & xx.xx \\
& Scene1 & xx.xx & xx.xx & xx.xx & xx.xx & xx.xx & xx.xx \\
& Scene1    & xx.xx & xx.xx & xx.xx & xx.xx & xx.xx & xx.xx \\
\midrule
\multirow{3}{*}{T\&T}
& Scene1 & xx.xx & xx.xx & xx.xx & xx.xx & xx.xx & xx.xx \\
& Scene1 & xx.xx & xx.xx & xx.xx & xx.xx & xx.xx & xx.xx \\
& Scene1 & xx.xx & xx.xx & xx.xx & xx.xx & xx.xx & xx.xx \\
& Scene1    & xx.xx & xx.xx & xx.xx & xx.xx & xx.xx & xx.xx \\
\midrule
\multirow{3}{*}{D\&B}
& Scene1 & xx.xx & xx.xx & xx.xx & xx.xx & xx.xx & xx.xx \\
& Scene1 & xx.xx & xx.xx & xx.xx & xx.xx & xx.xx & xx.xx \\
& Scene1 & xx.xx & xx.xx & xx.xx & xx.xx & xx.xx & xx.xx \\
& Scene1    & xx.xx & xx.xx & xx.xx & xx.xx & xx.xx & xx.xx \\
\bottomrule
\end{tabular}
\caption{perscene}
\label{tab:random_like_whiteboard}
\end{table*}
